# Supplementary material for: A Policy Gradient Algorithm for the Risk-Sensitive Exponential Cost MDP
Source: arXiv:2202.04157 source file (2022-08-29)
Supplement: Supplementary file 1 [file limitCvar.tex]

Fix a policy and suppose that the probability transition, under this policy, from any state $y$ to another state $z$ is perturbed from $p(z|y)$ to $p(z|y)\delta(z|y),$ where $\delta$ is a perturbation factor. Then it has been shown in \cite{chow2015risk} that, over a finite horizon $T,$ the CVaR-based controller is robust to perturbations which satisfy $\delta(x_2|x_1)\ldots\delta(x_T|x_{T-1})\leq \gamma$, $\forall x_1,\ldots x_T$ where $\gamma>1$ is a parameter associated with the CVaR metric and $x_t$ is the state at time $t.$ However, such a robustness criterion is not useful in many practical applications as we discuss next.

We consider a data center with a number of servers where the problem is to schedule arriving jobs on the servers. Such problems are important examples of the practical application of RL; see \cite{mao2019learning}, for example. Suppose that there are jobs of multiple types and whenever a job is rejected because of lack of capacity in the system, the revenue associated with that job is lost. Thus, the state of the MDP is the job occupancy in the data center and an indicator function which indicates whether or not there is an arrival in a time slot. Suppose we design an RL-based scheduling algorithm using traffic traces from the data center. The traffic traces will be associated with some arrival rates of jobs but when the RL algorithm is deployed in the data center, the rate at which jobs arrive to the system may be different. Consider a situation in which the arrival rate for one class of jobs is higher than in the training data set, then it is not hard to see then that $\delta(z|y)>1$ for some states. In this case, $\delta(x_2|x_1)\ldots\delta(x_T|x_{T-1})$ will be greater than $\gamma$ for many possible choices of $x_1$ through $x_T$ and therefore, the robustness guarantee provided by CVaR is not useful. We also note that, as the horizon increases, the perturbation constraint is more easily violated.
